# Supplementary material for: DeepXML: A Deep Extreme Multi-Label Learning Framework Applied to Short Text Documents
Source: arXiv:2111.06685 source file (2021-11-12)
Supplement: Supplementary file 1 [file results_q2b_supp.tex]

\begin{table*}[ht!]
\caption{Offline results on Q2B-3M. Methods marked with `-' refers to unavailable values.}
    \label{tab:sup:q2b_supp}
    \centering
    \resizebox{\textwidth}{!}{
    \begin{tabular}{@{}c|l|ccccc|ccccc|cc@{}}
    \toprule
    \textbf{Dataset} & \textbf{Method} & \textbf{P@1} & \textbf{P@3} & \textbf{P@5} & \textbf{N@3} & \textbf{N@5} &  \textbf{PSP@1} & \textbf{PSP@3}& \textbf{PSP@5} & \textbf{PSN@3} & \textbf{PSN@5}
    & \multicolumn{1}{c}{\begin{tabular}[c]{@{}c@{}}\textbf{Model}\\ \textbf{Size (GB)}\end{tabular}}
    & \multicolumn{1}{c}{\begin{tabular}[c]{@{}c@{}}\textbf{Training}\\ \textbf{Time (hr)}\end{tabular}} \\
    \midrule
  \multirow{7}{*}{\textbf{\rotatebox{90}{Q2B-3M}}}	& \alg	 & \textbf{73.37}	 & \textbf{33.91}	 & \textbf{21.67}	 & \textbf{83.52}	 & \textbf{85.13}	 & \textbf{64.8}	 & \textbf{85.13}	 & \textbf{90.42}	 & \textbf{79.1}	 & \textbf{81.24}	 & 15.7	 & 15.59 \\
	& Parabel	 & 54.29	 & 27.15	 & 17.94	 & 64.56	 & 66.98	 & 43.09	 & 61.66	 & 68.61	 & 55.1	 & 58.07	 & 5.84	 & 3.52 \\
	& PfastreXML	 & 43.48	 & 22.41	 & 15.01	 & 51.72	 & 53.9	 & 41.56	 & 55.38	 & 60.48	 & 49.13	 & 51.11	 & 172.48	 & 87.89 \\
	& Slice+CDSSM	 & 53.23	 & 27.53	 & 18.56	 & 65.08	 & 68.26	 & 42.35	 & 64.51	 & 74.14	 & 56.94	 & 61.09	 & 4.16	 & 4.71	\\
	& Parabel-weighted	 & 43.82	 & 22.25	 & 14.97	 & 52.15	 & 54.61	 & 37.83	 & 53.19	 & 59.57	 & 47.26	 & 49.94	 & -	 & - \\
	& Seq2Seq	 & 28.25	 & 13.06	 & 8.02	 & 22.96	 & 21.7	 & 23.32	 & 17.59	 & 15.42	 & 21.31	 & 21.3	 & -	 & -	 \\
	& Simrank++	 & 52.7	 & 29.69	 & 19.33	 & 50.02	 & 48.82	 & 43.5	 & 41.67	 & 39.36	 & 45.71	 & 45.73	 & -	 & 25 \\
    \bottomrule
    \end{tabular}
    }
\end{table*}
